# Supplementary material for: Carbide: Highly Reliable Networks Through Real-Time Multiple Control Plane Composition
Source: arXiv:2005.11425 source file (2022-01-13)
Supplement: Supplementary file 1 [file appendix.tex]

% \section{Global DFA Construction}
% Specifically, 
% consider $P$ as an expression of intersection / union on regular expression
% path sets $P_1, P_2, \ldots,$. Each $P_k$ is expressed as an
% automata $M_k$ defined as a tuple $(\Sigma, S_k, F_k, s_{k}^0, \sigma_k)$.
% The alphabet $\Sigma=V$, \ie, the set of all the network devices.
% $S_k$ is the set of states. $F_k \subseteq S_k$ is the set of accept states. 
% $s_{k}^0$ is the initial state. $\sigma_k: S_k \times
% \Sigma \rightarrow S_k$ is the state transition function. 
% \qiao{do we use rejection state anywhere? sending to rejection state can just be
% interpreted as not exist in $\sigma_k$....: gives all the valid transitions while invalid
% transitions are omitted here.} Figure~\ref{} gives the automata for the waypoint
% path set defined in the example program in
% Figure~\ref{fig:dv-example-requirement}. \qiao{if no space, forget it.}

% $P_{k_1} \cap P_{k_2}$ is represented by the intersection of $M_{k_1}$ and
% $M_{k_2}$. Specifically, $M_{k_1} \cap M_{k_2} = (V, S_{k_1} \times
% S_{k_2}, F_{k_1} \times F_{k_2}, (s_{k_1}^0, s_{k_2}^0), \sigma_{\cap})$ where
% $\forall v \in V, (s_{k_1}', s_{k_2}') = \sigma_{\cap}((s_{k_1}, s_{k_2}),
% v))$ if and only if $s_{k_1}' = \sigma_{k_1}(s_{k_1}, v)$ and $s_{k_2}' =
% \sigma_{k_2}(s_{k_2}, v)$. $P_{k_1} \cup P_{k_2}$ is represented as $M_{k_1}
% \cup M_{k_2}$, which is the same as $M_{k_1} \cap M_{k_2}$ except that its set
% of accept states is $(F_{k_1} \times S_{k_2}) \cup (S_{k_1} \times F_{k_2})$.

% After constructing a
% DFA $M=(\Sigma, S_P, F_P, s_P^0, \sigma_P)$ for $P$, \DistVeri constructs
% a DFA for the intersection of $P$ and topology $G$. Specifically, 
% $M_{P, G} = (V, S_{P, G}, F_{P, G}, s_{P, G}^0, \sigma_{P, G})$,
% where $S_{P, G} = V \times S_P$, $F_{P, G} = V \times F_P$, and 
% $\forall v' \in \Sigma, (v', s') = \sigma_{P, G}((v, s), v')$
% if and only if (1) there exists a link $v \rightarrow v'$ in $G$, and (2)
% $\sigma_P(s, v') = s'$.

% \input{syntax}
